# Supplementary material for: Diversifying Content Generation for Commonsense Reasoning with Mixture of Knowledge Graph Experts
Source: arXiv:2203.07285 source file (2022-03-14)
Supplement: Supplementary file 1 [file 6appendix.tex]

\subsection{Baseline Introduction}
\label{sec:baseline}

\noindent\textbf{CVAE}~\cite{kingma2014auto}. It is a basic variational auto-encoder model. We generate diverse outputs by sampling different latent variables.

\vspace{0.02in}
\noindent\textbf{VAE-SVG}~\cite{gupta2018deep}. It is a conditional variational autoencoder (CVAE) based generative framework for paraphrase generation. It proposes to control the influence of the latent variable of CVAE to generate diverse sequence.

\vspace{0.02in}
\noindent\textbf{SELECTOR}~\cite{cho2019mixture}.
It explicitly separates diversification from generation using a general plug-and-play module. The diversification stage also used a mixture of experts (MoE) module to sample different binary masks on the source sequence and generate diverse outputs.

\begin{figure*}[t]
    \centering
    {\includegraphics[width=1.0\textwidth]{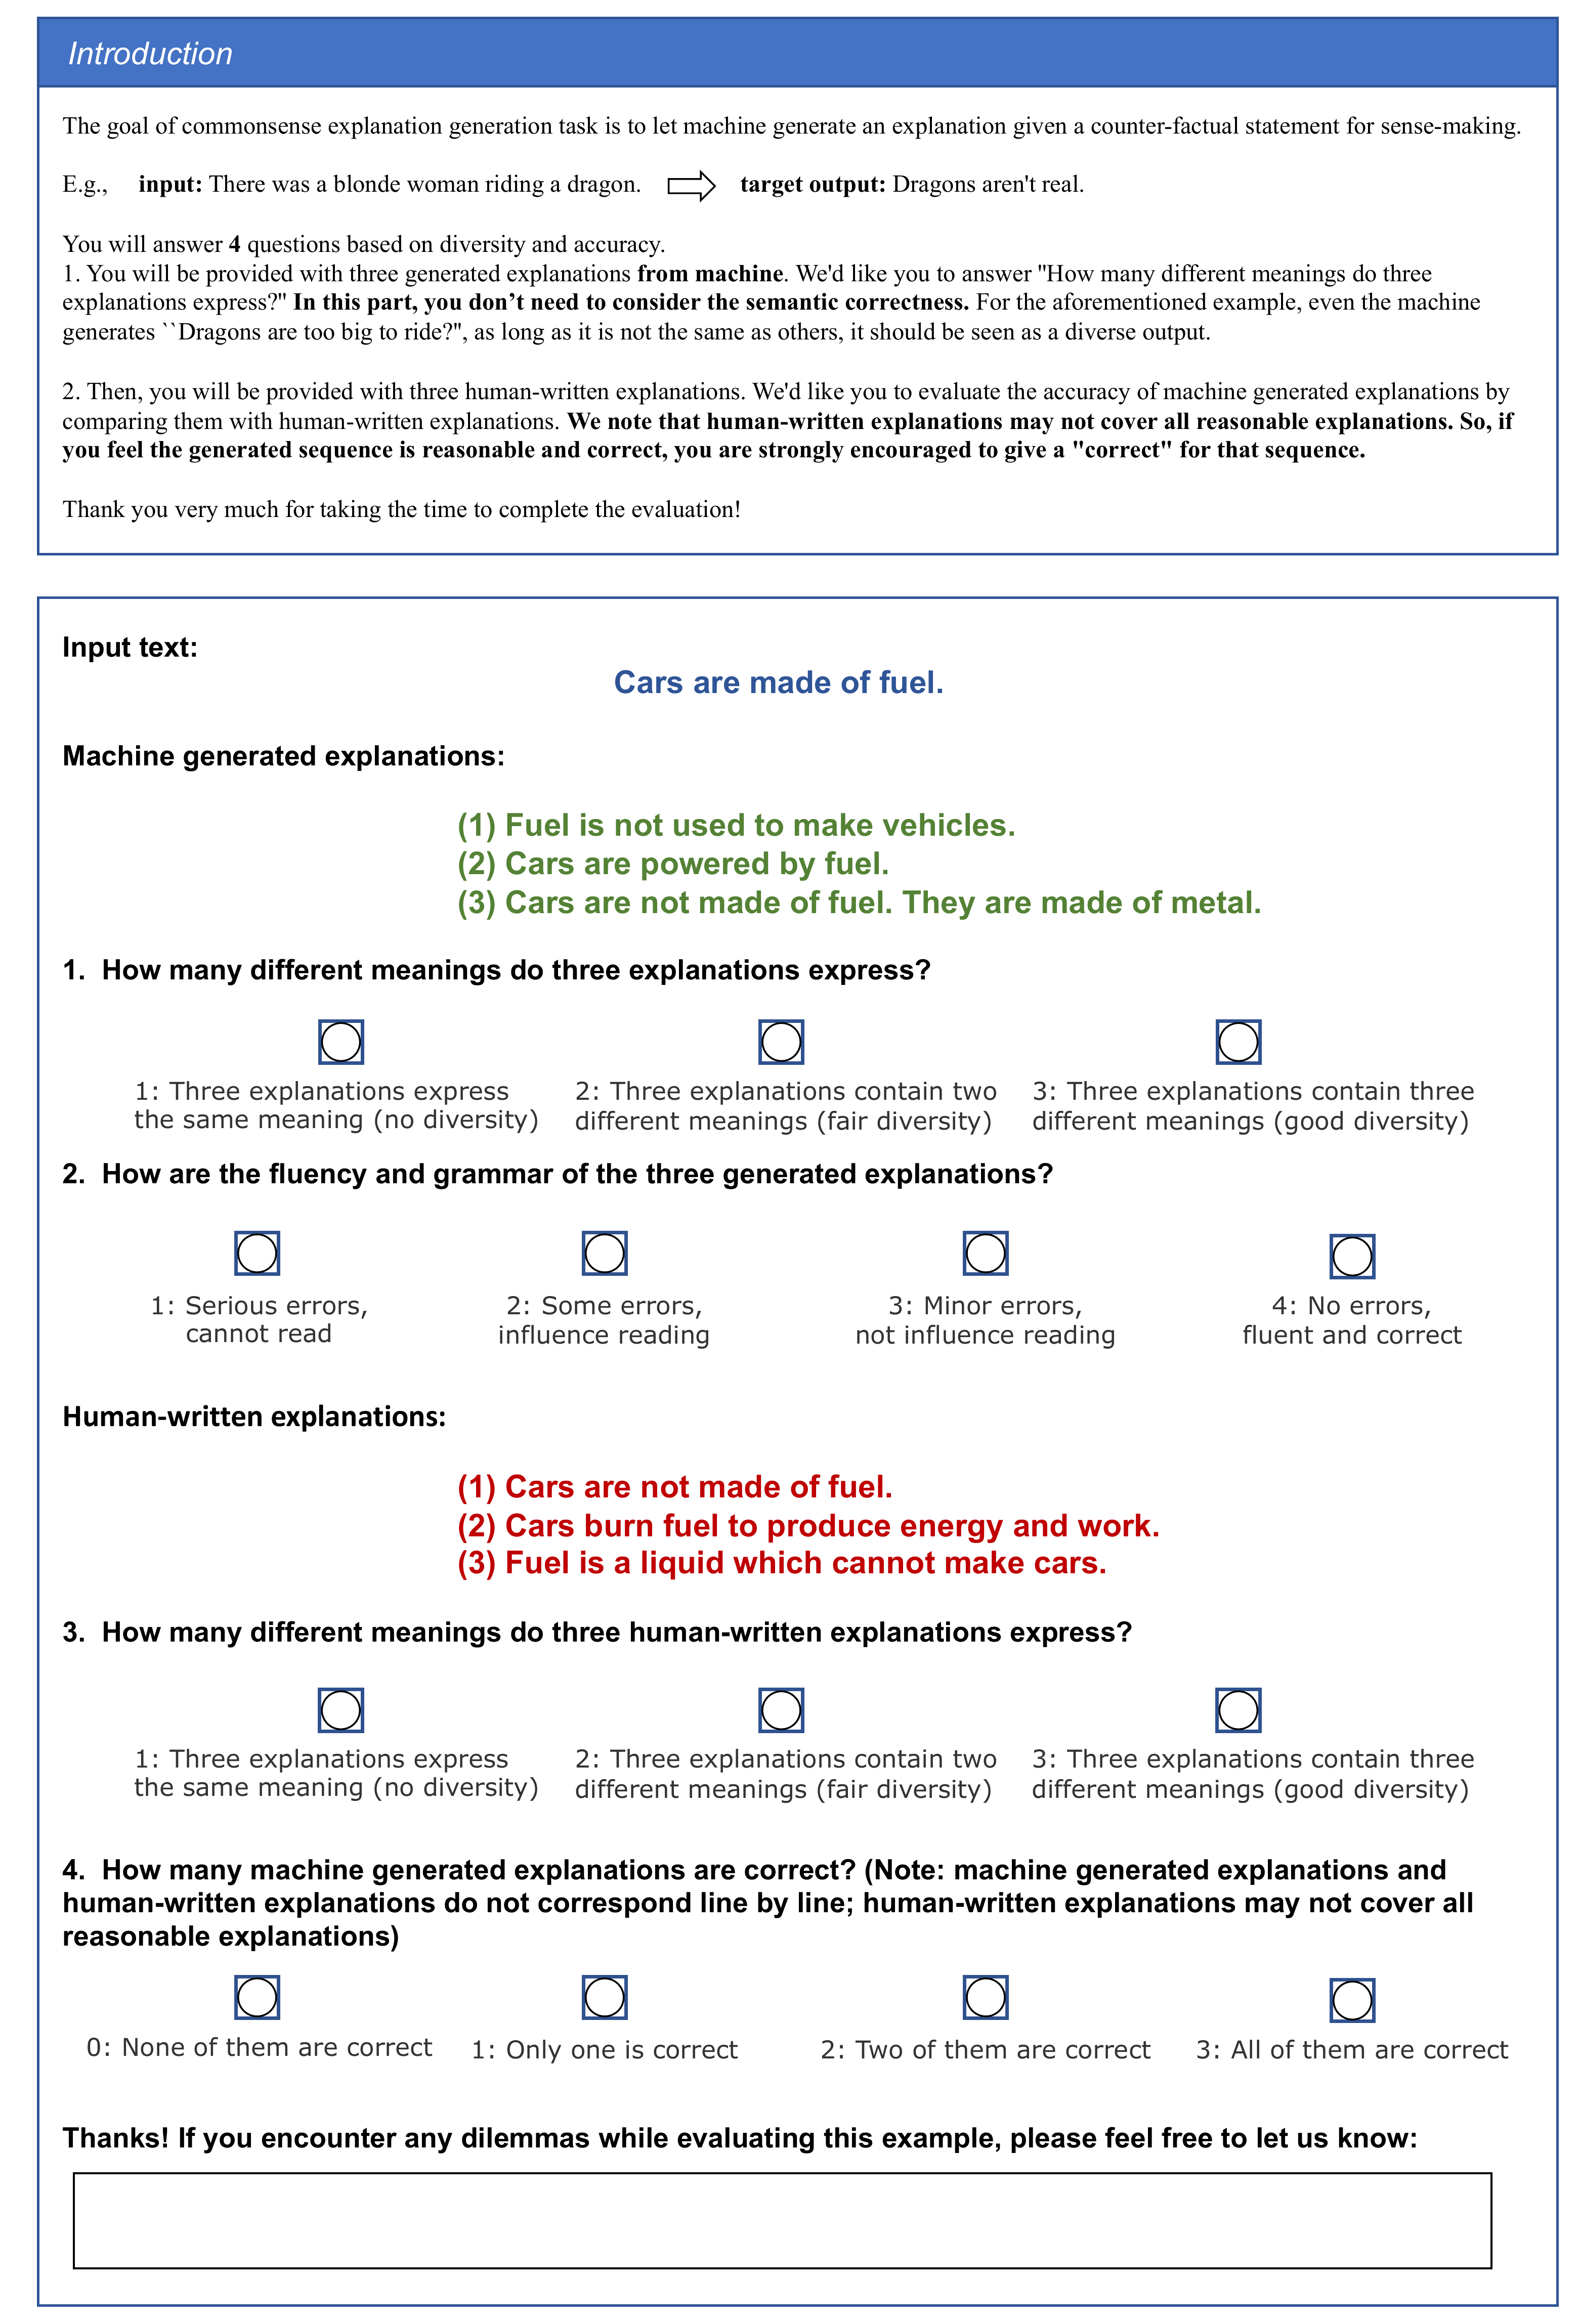}}
    \vspace{-0.2in}
    \caption{Human evaluation form. The example is from ComVE dataset.}
    \label{fig:human}
\end{figure*}

\subsection{Additional Dataset Statistics}
\label{sec:datasets}

We provide data statistics of ComVE~\cite{wang2020semeval} and $\alpha$-NLG~\cite{bhagavatula2020abductive}.
\vspace{-0.05in}

\begin{table}[h]
\caption{Statistics of two GR datasets.}
\vspace{-0.15in}
\begin{center}
\setlength{\tabcolsep}{6mm}{
\scalebox{0.85}{\begin{tabular}{l|c|c}
\toprule
Dataset & ComVE & $\alpha$-NLG \\
\midrule
\# Train & 50,481 & 10,000  \\
\# Dev. & 1,779 & 997  \\
\# Test & 3,560 & 1,000 \\
\# In.words & 7.7 & 17.4 \\
\# Out.words & 9.0 & 10.8 \\
\bottomrule
\end{tabular}}}
\label{tab:datasets}
\end{center}
\end{table}

\subsection{Other Baseline Methods}
\label{sec:other-base}

As we target at the \textit{one-to-many} generation problem, we exclude those baseline methods that cannot produce multiple outputs in the experimental section. We only list their quality performance in the following two tables (Table \ref{tab:b1}-\ref{tab:b2}). The evaluation process is based on only one output.

\begin{table}[h]
\caption{ComVE competition leaderboard.}
\vspace{-0.15in}
\begin{center}
\setlength{\tabcolsep}{3mm}{
\scalebox{0.85}{\begin{tabular}{clccc}
\toprule
Rank & Team / Paper & BLEU & Venue & Code \\
% \midrule
% \rowcolor{gray!12}\multicolumn{5}{c}{Participating teams} \\
\midrule
1 & (T) BUT-FIT & 22.4 & n/a & $\times$ \\
2 & (T) Solomon & 19.3 & n/a & $\times$ \\
3 & (T) KaLM & 18.5 & n/a & $\times$ \\
\rowcolor{gray!12} 4 & (O) MixKGE & 17.6 & - & - \\
5 & (P) GRF & 17.2 & EMNLP & $\surd$ \\
6 & (P)CE-PR & 16.9 & AACL & $\surd$ \\ 
7 & (T) panaali & 16.1 & n/a & $\times$ \\
8 & (T) cdjhz & 16.0 & n/a & $\times$ \\
% \midrule
% \rowcolor{gray!12}\multicolumn{5}{c}{Conference papers} \\
% \midrule
\bottomrule
\end{tabular}}}
\label{tab:b1}
\end{center}
\vspace{-0.05in}
\end{table}

\begin{table}[h]
\caption{SOTA performance on $\alpha$-NLG.}
\vspace{-0.15in}
\begin{center}
\setlength{\tabcolsep}{2mm}{
\scalebox{0.85}{\begin{tabular}{clccc}
\toprule
Rank & Paper & BLEU & Venue & Code \\
\midrule
1 & On-the-fly Attn & 13.5 & arXiv & $\times$ \\
\rowcolor{gray!12} 2 & MixKGE & 12.4 & - & - \\
3 & GRF & 11.6 & EMNLP & $\surd$ \\
4 & GPT2-OMCS & 9.6 & OpenAI Blog & $\surd$ \\
\bottomrule
\end{tabular}}}
\label{tab:b2}
\end{center}
\end{table}

\subsection{Implementation Details}
\label{sec:imple-details}

We implemented CVAE, VAE-SVG and SELECTOR by using the original codes from their github repositories. These three methods are based on the RNN-Seq2Seq~\cite{sutskever2014sequence} framework.

For truncated sampling and nucleus sampling, we used the BART-base~\cite{lewis2019bart} as the base model since BART is one of the state-of-the-art pre-trained generation models~\cite{gehrmann2021gem}.

In our MixKGE, the Transformer parameters were also initialized by BART-base, in order to make fair comparison with truncated sampling and nucleus sampling. The GNN parameters are were random initialized.

The Transformer took a maximum 512 input token sequence and consists of a 6-layer transformer encoders and another 6-layer transformer decoders~\cite{vaswani2017attention} with 12 attention heads and 768 word dimensions. For model fine-tuning, we used Adam with learning rate of 3e-5, L2 weight decay of 0.01, learning rate warm up over the first 10,000 steps, and linear decay of learning rate. Our models were trained by one Tesla V100 GPU card with 32GB memory, and implemented on PyTorch with the Huggingface's Transformer~\cite{wolf2020transformers}.
All Transformer-based methods were trained with 25 epochs.

\subsection{Experiments on Different Number of Experts}
\label{sec:number-experts}

We varied the number of experts to generate different number of outputs. In order to make fair comparisons, for truncated sampling and nucleus sampling, we changed the beam number to generate the same amount of output as MixKGE.

\begin{table}[h]
\caption{MixKGE consistently outperforms sampling based methods with different number of outputs based on diversity evaluation.}
\vspace{-0.15in}
\begin{center}
\setlength{\tabcolsep}{1mm}{
\scalebox{0.81}{\begin{tabular}{l|cc|cc}
\toprule
{\multirow{2}*{Methods}} & \multicolumn{2}{c|}{ComVE} & \multicolumn{2}{c}{$\alpha$-NLG}  \\
& S-BLEU($\Downarrow$) & BLEU($\Uparrow$) & S-BLEU($\Downarrow$) & BLEU($\Uparrow$) \\
\midrule
\rowcolor{gray!12}\multicolumn{5}{c}{Number of outputs = 4} \\
\midrule
Truncated & 0.7976 & 0.1702 & 0.7219 & 0.1346 \\
Nucleus & 0.7953 & 0.1693 & 0.7360 & 0.1362 \\
MixKGE & 0.3491 & 0.1694 & 0.2437 & 0.1222 \\
\midrule
\rowcolor{gray!12}\multicolumn{5}{c}{Number of outputs = 5} \\
\midrule
Truncated & 0.8321 & 0.1778 & 0.7674 & 0.1396 \\
Nucleus & 0.8311 & 0.1732 & 0.7761 & 0.1401 \\
MixKGE & 0.3940 & 0.1720 & 0.2739 & 0.1283 \\
\bottomrule
\end{tabular}}}
\label{tab:a4}
\end{center}
\end{table}

As shown in Table \ref{tab:a4}, when increasing the number of experts in MixKGE and beams in sampling methods, the generation quality does not have much change. For generation diversity, our proposed MixKGE can consistently outperform sampling methods by a large margin. Besides, we note that since Self-BLEU measures similarity between all pairwise combinations, the evaluation results will naturally increase when the number of generated outputs increases, so the Self-BLEU between different number of outputs is not comparable.

\subsection{Experiments on Expert Regularization}
\label{sec:experts-regu}

Ideally, we would like different experts to specialize in different reasoning abilities, so they can generate diverse outputs. In practice, however, different experts may still choose very similar groups of concepts. Therefore, we conducted experiments to compare the model performance between MixKGE (w/o rule) and adding heuristic rules on MixKGE (with rule) to constrain different experts to choose different concepts (without overlapping concepts).

\begin{table}[h]
\caption{MixKGE consistently outperforms.}
\vspace{-0.15in}
\begin{center}
\setlength{\tabcolsep}{1mm}{
\scalebox{0.81}{\begin{tabular}{c|cc|cc}
\toprule
{\multirow{2}*{Methods}} & \multicolumn{2}{c|}{ComVE} & \multicolumn{2}{c}{$\alpha$-NLG}  \\
& S-BLEU($\Downarrow$) & BLEU($\Uparrow$) & S-BLEU($\Downarrow$) & BLEU($\Uparrow$) \\
\midrule
w/o rule & 0.2423 & 0.1761 & 0.2159 & 0.1238 \\
with rule & 0.2108 & 0.1468 & 0.1841 & 0.1001 \\
\bottomrule
\end{tabular}}}
\label{tab:a5}
\end{center}
\end{table}

As shown in Table \ref{tab:a5}, we observe that adding the heuristic rule to avoid choosing overlapping concepts on the KG can further improve the generation diversity, but the quality has decreased significantly compared to the original MixKGE setting.

There are two main reasons causing this phenomenon. First, having a small portion of overlapping concepts between two outputs does not mean that they have the same meaning. Second, compared to the MixKGE, adding this rule can bring more irrelevant concepts to the generation process.

\subsection{Human Evaluation Form}
The human evaluation form is shown in Figure \ref{fig:human}.
